# Supplementary material for: Reproducibility and Artifact Consistency of the SIGIR 2022 Recommender Systems Papers Based on Message Passing
Source: arXiv:2503.07823 source file (2026-03-27)
Supplement: Supplementary file 1 [file Appendix_reproducibility.tex]

\clearpage
\section{Reproducibility summary}
\label{sec:reproducibility_summary}

Summary of the reproducibility of each experiment along different dimensions.
\begin{description}
    \item[Original hyp.] Whether we are using the hyperparameters as described in the article. Cases in which we use hyperparameters taken from the Github code are explicitly highlighted with a "No" or "-" depending on how critical they are. 
    \item[Dataset stats] Whether the dataset statistics we obtain (users, items, interactions) are consistent with the ones reported in the original paper.
    \item[Original split] Whether we are using the original split provided by the authors. If the data is splitted using the timestamp, that is explicitly indicated as it guarantees the validation data to be consistent as well. A hidden issue is the absence in most cases of the negative items when the algorithms are evaluated with the k-positives against h-negatives. Their absence means that even if the original test interactions are provided, the test data we have is not complete and therefore cannot be consistent with the original one, so the results are not directly comparable.
    \item[Reproducible] Whether the results we get are consistent to what reported in the original paper. "Yes" means they are very close, "Lower" and "Higher" means that we get respectively lower or higher results than what reported in the original paper, but even if we were to use the results in the original paper that would NOT impact the relative ordering of algorithms or our conclusions. "No" means that we get different results and using the original ones would change the experiment outcome.
\end{description}

\begin{table}[h]
\resizebox{.8\linewidth}{!}{%
    \begin{minipage}{\textwidth}
    \begin{tabular}{cl|cccc}
    \toprule
    Algorithm   & Dataset       & Original hyp.	&  Dataset stats     & Original split	 & Reproducible	\\ 
    \midrule
    \multirow{3}{*}{CMN}  	
        		&Epinions	    & Yes 	            & Yes 	            & No                 & No \footnote{Our results are -0.1 (75\%) on HR. Original results would change the conclusion.}   \\ 
        		&citeulike-a	& Yes 	            & Yes               & Yes 	             & Yes   \\ 
        		&Pinterest	    & Yes 	            & Yes 	            & Yes 	             & Yes	 \\ 
    \midrule
    \midrule
    \multirow{4}{*}{SpectralCF}  	
        		&Movielens1M   & Yes 	            & Yes 	            & Yes                & Yes  \\ 
        		&Movielens1M   & Yes 	            & Yes               & No 	             & - %\footnote{Our results are +0.1 (120\%) on Recall but -0.04 (60\%)on MAP}  
        		\\ 
        		&HetRec ML	   & Yes 	            & Yes               & No 	             & - %\footnote{Our results are +0.03 (111\%) on Recall but -0.02 (90\%)on MAP}   
        		\\ 
        		&Amazon Video  & Yes 	            & Yes 	            & No 	             & Higher %\footnote{Our results are +0.07 (120\%) on Recall and +0.007 (140\%) on MAP}	
        		\\ 
    \midrule
    \midrule
    \multirow{1}{*}{MCRec}  	
        		&ML100k   & - \footnote{Missing layer size, using github value}	  & - 	            & Yes                & Lower \footnote{Our results are 10\% lower. Original results would NOT change the conclusion.}  \\ 
    \midrule
    \multirow{2}{*}{CVAE}  	
        		&citeulike-a   & Yes 	            & Yes 	            & Yes                & - \footnote{\label{foot:repr_stat_metrics_wrong}Metrics implemented in original paper are wrong} \\ 
        		&citeulike-t   & Yes 	            & Yes 	            & Yes                & Yes  \\ 
    \midrule
    \multirow{2}{*}{CDL}  	
        		&citeulike-a   & Yes 	            & Yes 	            & Yes                & - \footnoteref{foot:repr_stat_metrics_wrong} \\ 
        		&citeulike-t   & Yes 	            & Yes 	            & Yes                & Yes  \\ 
    \midrule
    \midrule
    \multirow{2}{*}{NeuMF}  	
        		&ML1M           & Yes 	            & Yes 	            & Yes                & Yes \footnote{Our results are 5\% lower on HR. Original result would change the conclusion, but as per Xiangnan attempts still NeuMF is not consistently competitive (if we change the earlystopping as well)}  \\ 
        		&Pinterest      & Yes 	            & Yes 	            & Yes                & Yes  \\ 
    \midrule
    \multirow{2}{*}{Mult-VAE}  	
        		&ML20M          & Yes 	            & Yes 	            & Yes                & Lower  \\ 
        		&Netflix Prize  & Yes 	            & Yes	            & Yes                & Lower  \\ 
    \midrule
	\bottomrule
   	\end{tabular}
   	\end{minipage}
  	}
    \caption{Details on the reproducibility of algorithms from WWW, RecSys, KDD and SIGIR.}
    \label{tab:KNN_hyperparameters_our_baselines}
\end{table}

\begin{table}[h]
\resizebox{.8\linewidth}{!}{%
    \begin{minipage}{\textwidth}
    \begin{tabular}{cl|cccc}
    \toprule
    Algorithm   & Dataset       & Original hyp.	&  Dataset stats     & Original split	 & Reproducible	\\ 
    \midrule
    \multirow{2}{*}{DELF}  	
        		&Amazon Music   
        		& Yes 	            
        		& Yes 	            
        		& No, Timestamp (missing neg)                
        		& No \footnote{\label{foot:repr_stat_toppop_consistent} TopPop is consistent} \footnote{Our results are between -12\% and -5\%. This dataset has on avg 2 interactions per item, the validation split may result in cold items. The paper shows exponential improvement for HR at increasing embedding size and stops at 64. HR values for different cutoffs grows linearly, precision almost constant at cutoffs >5. Even considering the 4 negative items used in training, the algorithm has massively more parameters than data points. No regularization used, as confirmed by the authors. Epochs chosen with test data.}  
        		\\ 
        		&ML1M          
        		& Yes 	            
        		& Yes 	            
        		& No, Timestamp (missing neg)               
        		& Yes \footnote{Our results are 2\% to 4\% lower. Original results would NOT change the conclusion.}  \\
    \midrule
    \multirow{2}{*}{CoupledCF}  	
        		& ML1M      
        		& - \footnote{\label{foot:repr_stat_coupledcf}Convolution filter is stated to be (8,8) but in code is (3,3). (8,8) is an uncommonly huge number. No reply to enquiry.}	            
        		& Yes 	            
        		& Yes, neg included               
        		& Yes / No %\footnote{\label{foot:repr_stat_NDCG_wrong}NDCG is implemented wrong as 2 is added to the position of the hit instead of 1. } 
        		\footnote{DeepCF yes. CoupledCF is -12\% to -20\%. Original results would outperform baselines. No reply to requests. If we split the data ourselves the performance drops dramatically.} 
        		\\ 
        		& Tafeng\footnote{The split is wrong. 4\% of users having a test interaction are not associated to any negative item. A random recommender would have 100\% precision.}    
        		& - \footnoteref{foot:repr_stat_coupledcf} 	            
        		& Yes \footnote{Interaction number they declare is higher by more than 10\% but we are using their data split.} 	& Yes, neg included                
        		& Yes / Lower %\footnoteref{foot:repr_stat_NDCG_wrong} 
        		\footnote{DeepCF yes. CoupledCF is 5\% lower. Original results would NOT change our conclusion since 1 of 2 metrics is still lower than baselines.}  \\ 
    \midrule
    \multirow{4}{*}{NeuRec}  	
        		& ML Hetrec   & Yes \footnote{\label{foot:repr_stat_NeuRec_hyperp} Batch size not available} 	            
        		& Yes 	           
        		& No               
        		& No \footnoteref{foot:repr_stat_toppop_consistent} \footnote{\label{foot:repr_stat_non_repr_original_code} Results non reproducible even with original code.} \footnote{Our results are between -10\% and -27\%. Original result would change our conclusions.}
        		\\ 
        		& ML1M       
        		& Yes \footnoteref{foot:repr_stat_NeuRec_hyperp} 	           
        		& missing 	            
        		& No                
        		& - \footnoteref{foot:repr_stat_toppop_consistent} \footnoteref{foot:repr_stat_non_repr_original_code} \footnote{Our results are between -12\% and -50\%. Original result would NOT change our conclusions.}
        		\\ 
        		& Filmtrust   
        		& Yes \footnoteref{foot:repr_stat_NeuRec_hyperp} 	           
        		& missing 	            
        		& No                
        		& Yes / No \footnoteref{foot:repr_stat_toppop_consistent} \footnoteref{foot:repr_stat_non_repr_original_code} \footnote{INeuRec is reproducible. UNeuRec is -5\% to -10\%. Original result would NOT change our conclusions.}
        		\\ 
        		& Frappe      
        		& Yes \footnoteref{foot:repr_stat_NeuRec_hyperp} 	            
        		& missing 	            
        		& No                
        		& No \footnote{Results are completely different. TopPop is NOT consistent by far, 400\% the value reported in the original paper, NeuRec results are 200\% the value reported in the original paper.} 
        		\\ 
    \midrule
    \multirow{4}{*}{DMF}  	
        		&ML100k   
        		& Yes 	            
        		& Yes 	            
        		& No, Timestamp (missing neg)                
        		& No \footnoteref{foot:repr_stat_toppop_consistent} %\footnoteref{foot:repr_stat_NDCG_wrong}
        		\footnote{Our results are -10\%. Original result would change our conclusions.}
        		\\ 
        		&ML1M   
        		& Yes	            
        		& Yes 	            
        		& No, Timestamp (missing neg)                  
        		& No \footnote{TopPop is NOT consistent, our results are almost 10\% higher.} %\footnoteref{foot:repr_stat_NDCG_wrong}
        		\footnote{Our results are -10\%. Original result would change our conclusions.} 
        		\\ 
        		&Amazon Music   
        		& Yes 	            
        		& No \footnote{The authors provided a "pruned" version of the dataset smaller than what we obtain applying the described preprocessing.}	            
        		& No, Timestamp (missing neg)                  
        		& Yes \footnoteref{foot:repr_stat_toppop_consistent}   %\footnoteref{foot:repr_stat_NDCG_wrong}
        		\footnote{Our results are -5\%. Original result would NOT change our conclusions, algorithm is slightly competitive in 1 out of 2 metrics.} 
        		\\ 
        		&Amazon Movies   
        		& Yes 	            
        		& No \footnote{Applying the described preprocessing we get 15k users instead of 9k and 10\% more interactions.}	            
        		& No, Timestamp (missing neg)                  
        		& Higher \footnote{TopPop is NOT consistent, our results are almost 10\% higher.} %\footnoteref{foot:repr_stat_NDCG_wrong}
        		
        		\\ 
    \midrule
    \multirow{2}{*}{ConvNCF}  	
        		& Yelp  
        		& No \footnote{\label{foot:repr_stat_convncf_no_hyperp} Hyperparameters not described in article, using Github ones. The only two hyperp. in article are consistent with Github. No reply to enquiry. Xiangnan is an author.}	            
        		& No \footnote{Interaction number we get is 69k vs 730k.} 	            
        		& Yes, Timestamp (missing neg)                  
        		& Yes %\footnoteref{foot:repr_stat_NDCG_wrong} 
        		\footnote{TopPop not consistent, we get +3\%} 
        		\\ 
        		& Gowalla   
        		& No \footnoteref{foot:repr_stat_convncf_no_hyperp}	            
        		& Yes	            
        		& Yes, Timestamp (missing neg)                  
        		& Yes %\footnoteref{foot:repr_stat_NDCG_wrong} 
        		\footnote{TopPop not consistent, we get +10\%} 
        		\footnote{Our results are -3\%. Original result would NOT change our conclusions}
        		\\  
	\bottomrule
   	\end{tabular}
   	\end{minipage}
  	}
    \caption{Details on the reproducibility of algorithms from IJCAI.}
    \label{tab:KNN_hyperparameters_our_baselines}
\end{table}

\clearpage
